# Supplementary material for: Bridging Critical Gaps in Convergent Learning: How Representational Alignment Evolves Across Layers, Training, and Distribution Shifts
Source: arXiv:2502.18710 source file (2025-11-25)
Supplement: Supplementary file 1 [file inter-model-sm.tex]

\begin{figure}[htbp!]
    \centering
    % cifar100
    %\includegraphics[width=.16\textwidth]{figures/inter-model-analysis-results/resnet18_resnet50_soft_match_cifar100_comparison.png}\hfill
    %\includegraphics[width=.16\textwidth]{figures/inter-model-analysis-results/resnet18_vgg16_soft_match_cifar100_comparison.png}\hfill
    %\includegraphics[width=.16\textwidth]{figures/inter-model-analysis-results/resnet18_vgg19_soft_match_cifar100_comparison.png}\hfill 
    %\includegraphics[width=.16\textwidth]{figures/inter-model-analysis-results/vgg16_resnet50_soft_match_cifar100_comparison.png}\hfill
    %\includegraphics[width=.16\textwidth]{figures/inter-model-analysis-results/vgg19_resnet50_soft_match_cifar100_comparison.png}\hfill 
    %\includegraphics[width=.16\textwidth]{figures/inter-model-analysis-results/vgg16_vgg19_soft_match_cifar100_comparison.png}\\
    
    % imagenet
    \includegraphics[width=.16\textwidth]{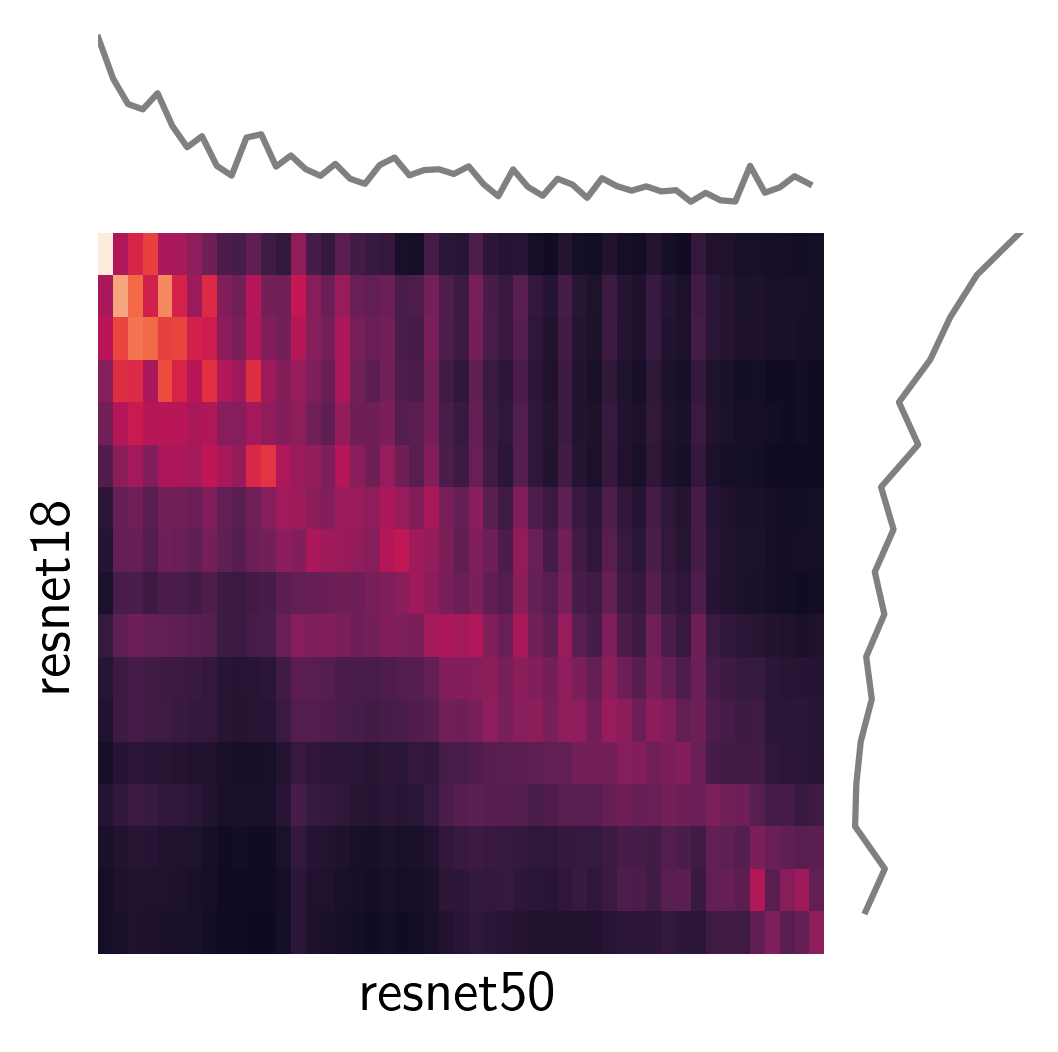}\hfill
    \includegraphics[width=.16\textwidth]{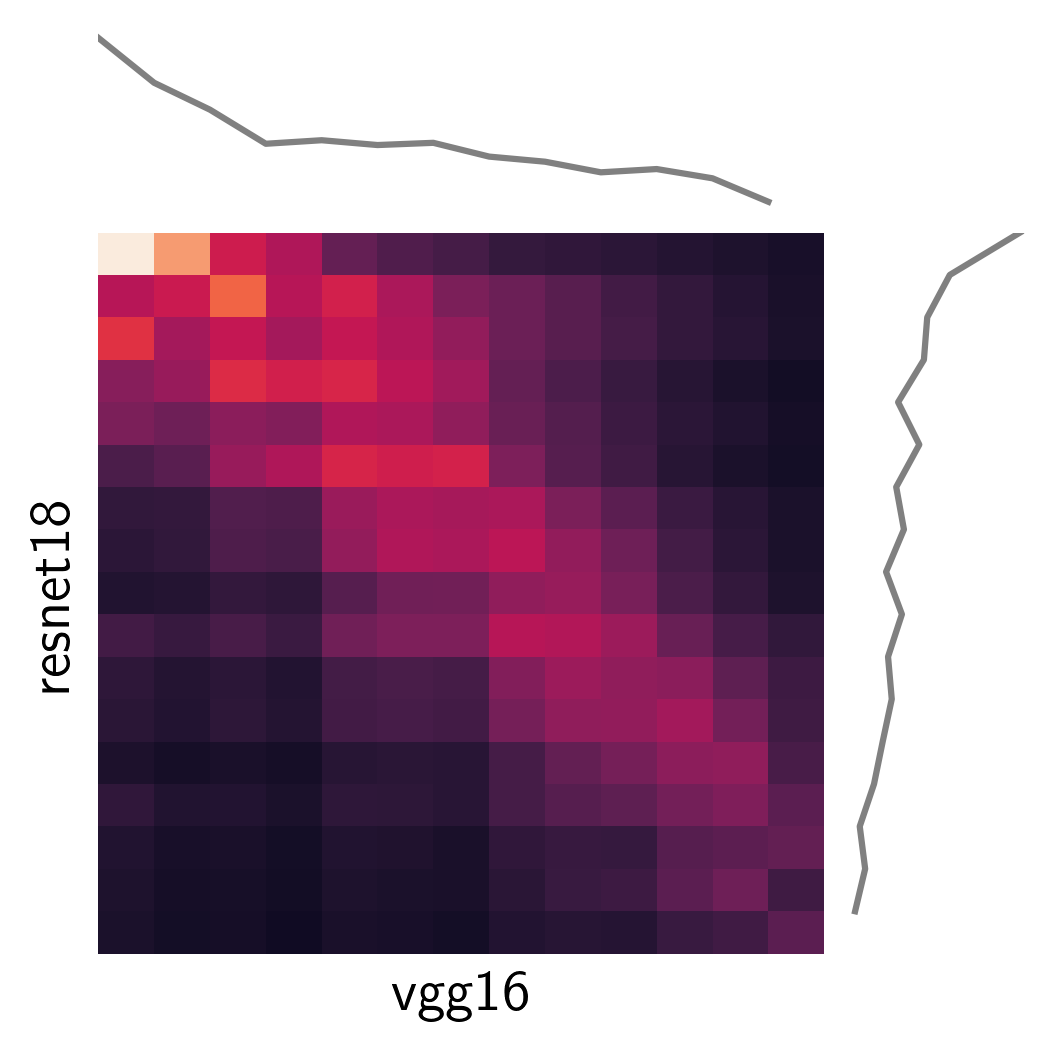}\hfill
    \includegraphics[width=.16\textwidth]{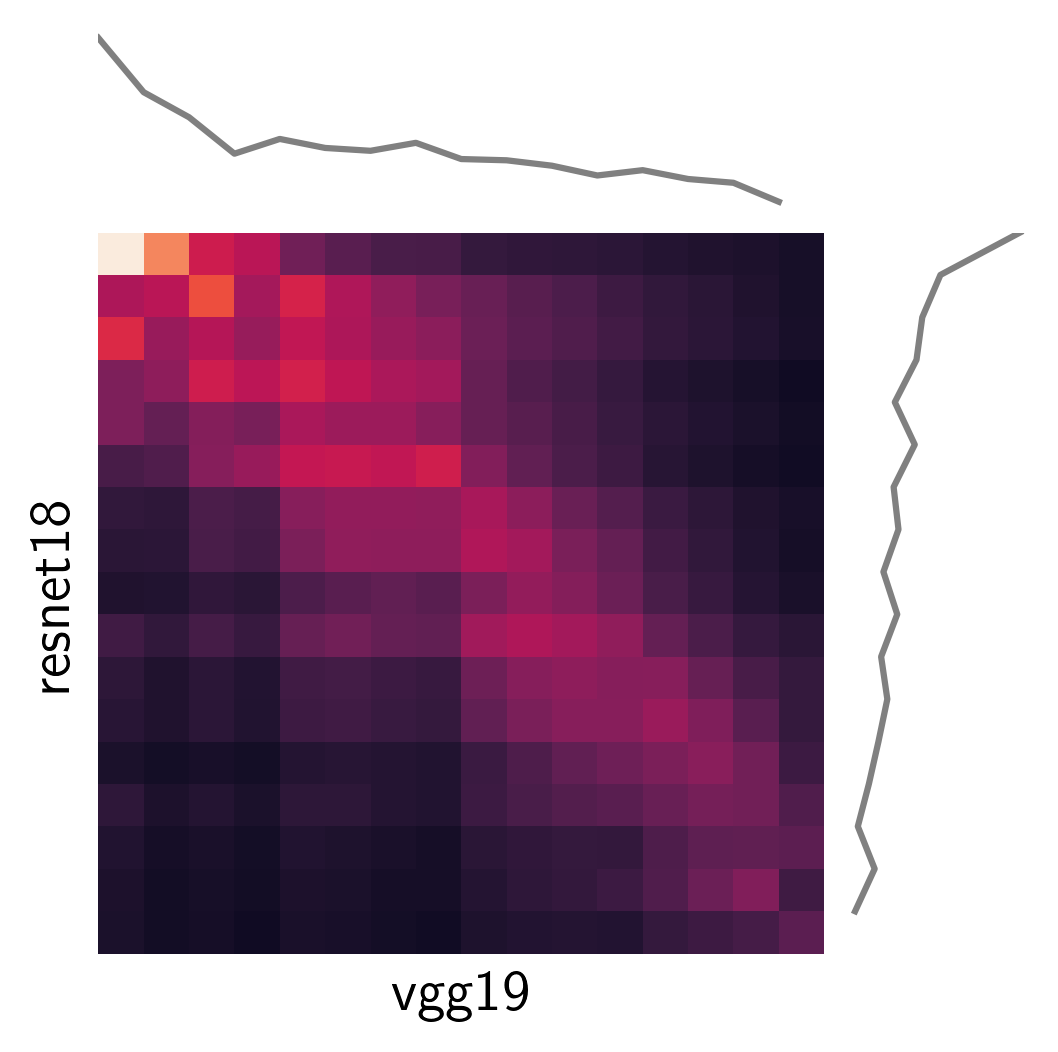}\hfill 
    \includegraphics[width=.16\textwidth]{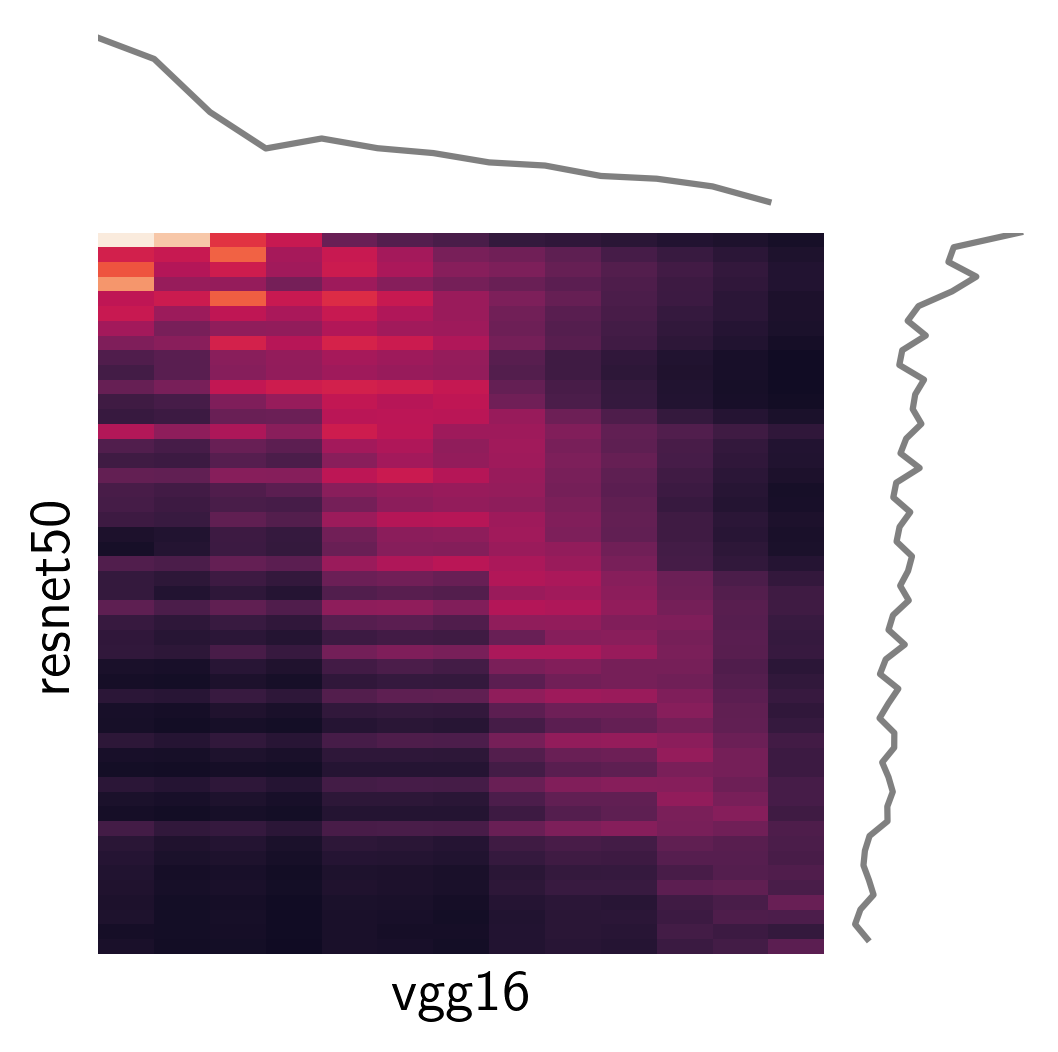}\hfill
    \includegraphics[width=.16\textwidth]{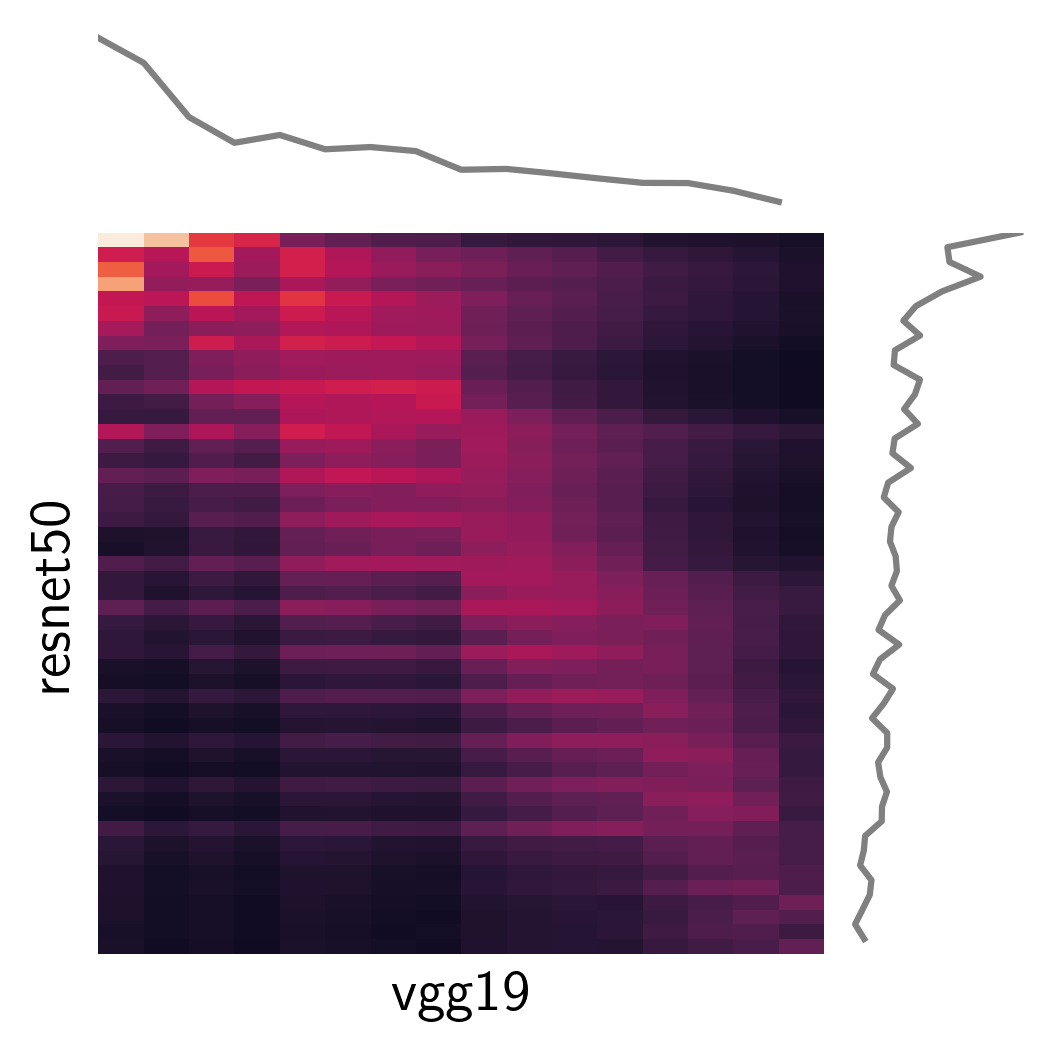}\hfill 
    \includegraphics[width=.16\textwidth]{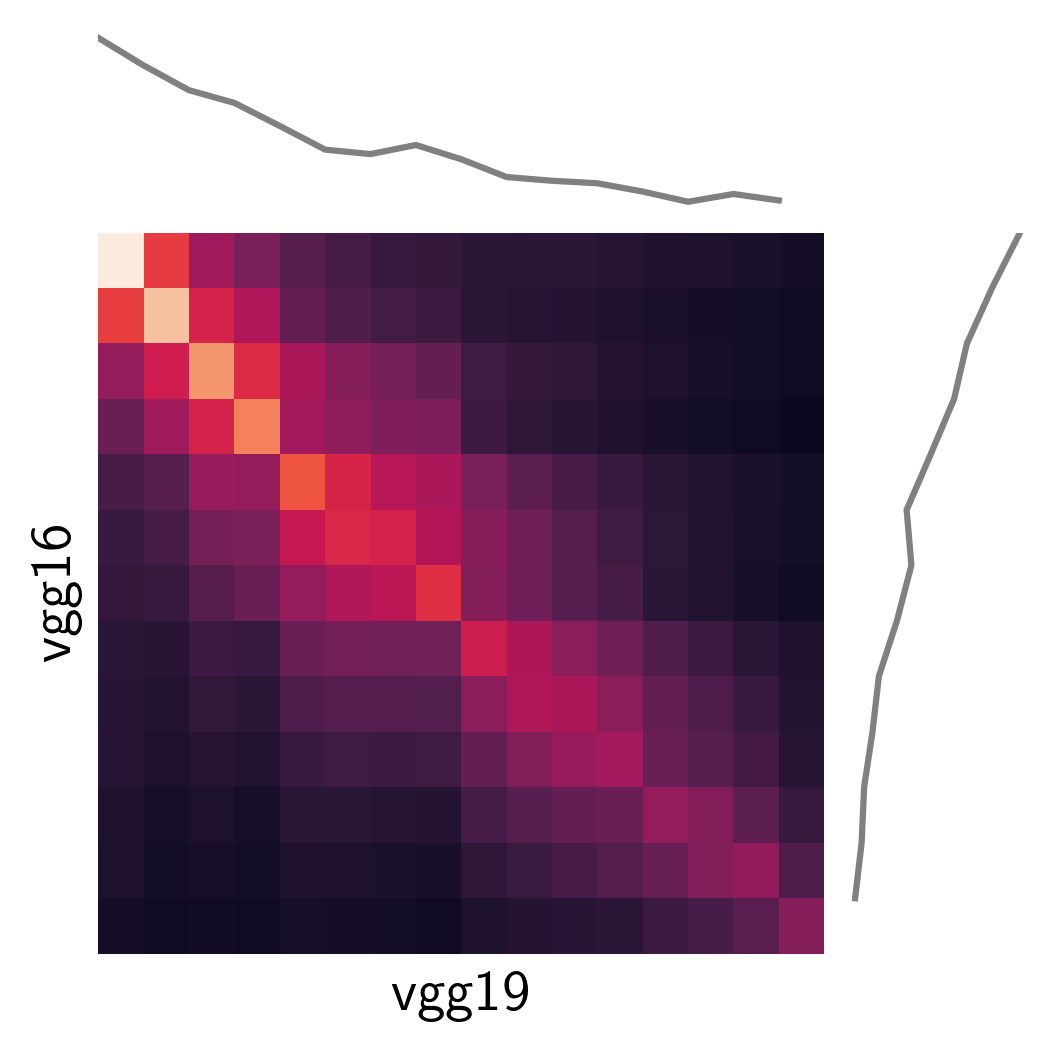}
    \caption{\textbf{Inter-Model Soft-Match.} Identical to the preceding plot, we compute the layer-wise soft-matching score for all networks pairs ImageNet, similarly revealing consistent inter-layer relationships across architectures.}
    
    \label{tab:sm_inter_model} 
\end{figure}
